# Supplementary material for: PrivacyProxy: Leveraging Crowdsourcing and In Situ Traffic Analysis to Detect and Mitigate Information Leakage
Source: arXiv:1708.06384 source file (2018-10-26)
Supplement: Supplementary file 1 [file 08_appendix.tex]

\clearpage
\begin{table*}
\section{Comparison with Recon And HayStack}
\label{sec:Appendix}
\vspace{4mm}
\small
\centering
\begin{adjustbox}{center, width=(\columnwidth-20pt) * 2}

\begin{tabular}{|c|c|p{3cm}|p{3cm}|p{5cm}|}
\cline{1-5}
\textbf{Package Name} & \textbf{Metrics} & \textbf{Recon}            & \textbf{HayStack}                & \textbf{PrivacyProxy} \\ 
\hline
\hline
\multirow{2}{*}{\centering com.ketchapp.ballz} & True Positives  & {\centering Email, Advertiser ID, Device ID} & {\centering Android Serial, Hardware Info} & {\centering User ID, Location, Request ID, Session ID, Google Advertiser ID}\\ 
\cline{2-5} 
& \centering False Positives\textsuperscript{1} & {\centering -} & {\centering Timezone, Build Fingerprint} & {\centering -} \\ \hline

\multirow{2}{*}{com.cmplay.tiles2} & True Positives  & {\centering Advertiser ID, Location, Android ID} & {\centering Android ID, Android Serial, Account, Hardware Info} & {\centering IDFA, Advertiser ID, Task Collected Advertiser ID, Session ID, Android ID, Social ID, First Launch Date, UID, Device Info, Channel ID, Install Date}\\ 
\cline{2-5} 
& \centering False Positives\textsuperscript{1} & {\centering -} & {\centering Build Fingerprint, Timezone} & {\centering Fetch Next Ad Time, Timestamp} \\ \hline

\multirow{2}{*}{com.enflick.android.TextNow} & True Positives  & {\centering Advertiser ID, Email, Device ID, Android ID} & {\centering Android ID, Android Serial}& {\centering Android UUID, Client ID, GPS ADID, Created At, Sent At}
\\ 
\cline{2-5} 
& \centering False Positives\textsuperscript{1} & {\centering -} & {\centering -} & {\centering Token} \\ \hline

\multirow{2}{*}{com.fortafygames.colorswitch} & True Positives & {\centering Advertiser ID, Location, Android ID, Device ID} & {\centering Advertiser ID, Android ID} & {\centering Device ID, Android ID, Advertiser ID, Device Free Bytes}
\\ 
\cline{2-5} 
& \centering False Positives\textsuperscript{1} & {\centering Gender} & {\centering -} & {\centering -} \\ \hline

\multirow{2}{*}{com.pinterest} & True Positives  & {\centering Advertiser ID, Location, Android ID, Email} & {\centering Android ID} & {\centering Pinterest Install ID, Pinterest Device Hardware ID}
\\ \cline{2-5} 
& \centering False Positives\textsuperscript{1} & {\centering Gender} &
{\centering Build Fingerprint} & {\centering Requests URI} \\ \hline

\multirow{2}{*}{com.pixelberrystudios.choices} & True Positives  & {\centering Advertiser ID, Location, Android ID, Device ID, Email} &{\centering Android ID, Android Serial, Hardware Info} & {\centering Advertiser ID, Signature, Android ID, Crashanalytics Advertising Token, IDFA, IA, API ID, Render Ad Time, Install Time}
\\ \cline{2-5} 
& \centering False Positives\textsuperscript{1} & {\centering -} &
{\centering MMS User Agent, Timezone, Build Fingerprint} & {\centering Fetch Next Ad Time, Timestamp} \\ \hline

\multirow{2}{*}{com.soundcloud.android} & True Positives  & {\centering Advertiser ID, Location, Android ID, Device ID, Android ID Hash, Advertiser ID Hash} & {\centering Android ID, Account, Hardware Info} & {\centering Android ID, Created At, Session ID, GPS ADID, Crashanalytics ID, Device ID}
\\ \cline{2-5} 
& \centering False Positives\textsuperscript{1} & {\centering -} & {\centering Build Fingerprint} & {\centering Timestamp} \\ \hline

\multirow{2}{*}{com.steam.photoeditor} & True Positives  & {\centering Advertiser ID, Advertiser ID Hash, Location, Android ID, Email} &{\centering Android ID, Hardware Info} & {\centering Data Request Module ID, IMEI, Unique ID, Go ID, A ID, HMAC ID, Android ID}
\\ \cline{2-5} 
& \centering False Positives\textsuperscript{1} & {\centering Gender} & {\centering Build Fingerprint} & {\centering Request Time} \\ \hline

\multirow{2}{*}{com.surpax.ledflashlight.panel} & True Positives  & {\centering Advertiser ID, Email, Location, Android ID, Device ID} &{\centering Android ID} & {\centering User ID, Install Date, First Launch Date, Advertiser ID, Android ID, UDID}
\\ \cline{2-5} 
& \centering False Positives\textsuperscript{1} & {\centering -} & {\centering Build Fingerprint} & {\centering Timestamp} \\ \hline

\multirow{2}{*}{com.turbochilli.rollingsky} & True Positives  & {\centering Advertiser ID, Location, Android ID, Device ID, Advertiser ID Hash, Email}  & {\centering Android ID} & 
{\centering Android ID, Device Info, IDFA, Gaid, Stats Ad Session Start, App Install Time}
\\ \cline{2-5} 
& \centering False Positives\textsuperscript{1} & {\centering -} & {\centering Timestamp} &{\centering Timestamp, Fetch Next Ad Time, \KB{+1?}} \\ \hline

\multirow{2}{*}{com.zhiliaoapp.musically} & True Positives  & {\centering Advertiser ID, Email, Location, Device ID} & {\centering Android ID, Android Serial, Account, Hardware Info} & {\centering Device ID, IDFA, Request ID}
\\ \cline{2-5} 
 & \centering False Positives\textsuperscript{1} & {\centering -} & {\centering Build Fingerprint} & \multicolumn{1}{|c|}{\centering Message Type, Access Token} \\ \hline

\multirow{2}{*}{com.zynga.crosswordswithfriends} & True Positives  & {\centering Advertiser ID, Email, Location, MAC Address, Android ID, Device ID, Advertiser ID Hash} & {\centering Android ID, Android Serial, Account, Hardware Info} & {\centering User ID, Android ID, Session Last At, Device ID, IDFA, Session ID}
\\ \cline{2-5} 
& \centering False Positives\textsuperscript{1} & {\centering -} & {\centering Private IP, Timezone, Build Fingerprint} & {\centering Timestamp, Session Length, Event Time} \\ \hline

\multirow{2}{*}{com.bitmango.go.wordcookies} & True Positives  & {\centering Email, Advertiser Id, Location, Advertiser ID Hash, Android ID, Device ID} & {\centering Android Serial, Android ID, Hardware Info} & {\centering User ID, Installed At, Device Info, IDFA}
\\ \cline{2-5} 
& \centering False Positives\textsuperscript{1} & {\centering Gender} & {\centering Build Fingerprint} & {\centering Timezone, Fetch Ad Next Time, StatsAdSession} \\ \hline

\multirow{2}{*}{ Total PII Count} & True Positives & {\centering 68} & 37 & {\centering 96}
\\ \cline{2-5} 
& {\centering False Positives\textsuperscript{1}} & {4} & {\centering 21} & 22\\ \hline
\end{tabular}

\end{adjustbox}

\end{table*}
